# Supplementary material for: Playable Environments: Video Manipulation in Space and Time
Source: arXiv:2203.01914 source file (2022-03-15)
Supplement: Supplementary file 1 [file supplementary_datasets.tex]

\section{Datasets}
\label{sec:datasets}
In this section we describe the proposed \emph{Minecraft} and \emph{Tennis} datasets for the training of playable environments in in Sec.~\ref{sec:minecraft_dataset} and in Sec.~\ref{sec:tennis_dataset} respectively. We also present details for the \emph{Minecraft Camera} dataset in Sec.~\ref{sec:minecraft_camera_dataset} and the \emph{Static Tennis} dataset in Sec.~\ref{sec:static_tennis_dataset}.

\subsection{Minecraft dataset}
\label{sec:minecraft_dataset}

We collect videos where two \emph{Minecraft} players perform a sparring session. To acquire the sequences we build a Minecraft 16.4 \cite{minecraft} plugin based on \cite{replaymod} (GNU GPL v3). The plugin records Minecraft playing sessions and provides a GUI to replay the recorded sessions and render them under arbitrary camera trajectories. In addition, it is possible to re-render each sequence using different sets of textures for the environment and the players. Our plugin complements the rendered video with metadata containing camera intrinsic and extrinsic parameters and information about the entities that are present in the scene (eg. players). We release the code for the modified plugin to foster the use of Minecraft as a research tool.

We acquire sequences under varying illumination conditions where the camera slowly circles in a dome around the sparring area. Scenes at both day and night are recorded. The training set is composed of 69,600 frames in 1024x576 resolution at 20fps, divided in sequences of 400 frames. The test set and the validation set are composed each of 2,960 frames in sequences of 16 frames at 5fps. A total of 16 unique player identities are present. Note that the dataset can be automatically re-generated at arbitrary resolution and framerate.

\subsection{Minecraft Camera dataset}
\label{sec:minecraft_camera_dataset}

In order to evaluate the camera manipulation capabilities of our method, we collect additional \emph{Minecraft} sequences. In each sequence, the camera starts from an initial pose and is then moved in the neighborhood of the original position in a circular pattern to synthesize novel views of the scene. To allow a better evaluation of novel view synthesis, the rendered scene remains unchanged in all the frames. We collect 24 sequences, each of length 16 frames for a total of 384 frames. 

\subsection{Tennis dataset}
\label{sec:tennis_dataset}

\begin{table}
\begin{center}

\setlength{\tabcolsep}{2.0pt}
\footnotesize
\begin{tabular}{lccc}
\toprule
Tournament & Raw duration & Processed duration & Success \\
\midrule
Us Open & 23.090 & 20.912 & 90.6 \\
Australian Open & 12.267 & 11.778 & 96.0 \\
Wimbledon & 12.014 & 11.574 & 96.3 \\
Roland Garros & 8.448 & 1.205 & 14.3 \\
\midrule
Total & 55.819 & 45.469 & 81.5 \\

\bottomrule
\end{tabular}
\end{center}
\caption{Statistics on the collected \emph{Tennis} dataset indicating the duration of the collected raw sequences before camera calibration and player detection and the duration of the processed sequences for which camera calibration and player detection was performed successful. Success indicates the success rate in camera calibration and player detection. Dirt on the tennis lines causes a low success rate for Roland Garros sequences. Durations in seconds, success rate in \%.} 
%\vspace{-3mm}
\label{table:tennis_dataset_statistics}
\end{table}

We build a dataset of tennis match videos collected from YouTube. We collect a total of 43 tennis matches, featuring 86 different player appearances. The matches come from the following tournaments: 13 Us Open matches played on a concrete field, 7 Australian Open matches played on a concrete field, 8 Wimbledon matches played on grass, 15 Roland Garros matches played on red ground.
In each original video, we extract portions of the match where the game is actively being played, from the moment of the service to the realization of the point, and discard parts where no action is occurring. We then process such raw sequences to extract camera calibration information and player bounding boxes.

To perform camera calibration, we exploit the known geometry of the tennis field, using the field itself as a calibration pattern. To detect landmarks on the tennis field, we follow \cite{farin2003robustcameracalibration} using the implementation provided in \cite{implementationfarin2003robustcameracalibration} (BSD 3-Clause). Note that camera parameters obtained in this way present noise due to imprecision in the estimation of landmarks on the tennis field. We discard sequences with implausible camera poses or where camera calibration is excessively noisy using variance in the estimated camera position on the field as a noise estimator. In some sequences, camera calibration fails due to the inability to correctly detect the landmarks. This often happens in sequences from Roland Garros where the field lines are frequently covered by red ground and causes a high number of sequences from Roland Garros to be discarded. When possible, we provide camera parameters estimations for frames where landmark detection fails by interpolating the camera parameters of neighboring frames.

To perform player detection, we make use of a pretrained FasterRCNN \cite{ren2015faster} model. We employ the camera calibration parameters obtained in the preceding step to discard detections associated with people other than the players, \emph{i.e.} referees, ball catchers and spectators. We notice that detection is sometimes inaccurate or fails due to the wide range of movements performed by the players. This happens more frequently for the player positioned further from the camera. Similarly to camera calibration, we discard sequences where detection of one of the players presents an excessive number of failures. When possible, in case of failed detections in one frame, we interpolate the detections of neighboring frames to produce an estimated detection.

The sequences where both camera calibration and player detection complete successfully are selected to be part of the dataset. Tab.~\ref{table:tennis_dataset_statistics} shows the duration statistics for the raw sequences before camera calibration and player detection and for the sequences that were successfully processed. A total of 12.6 hours of videos at 5 fps and 512x288 resolution are successfully processed and are organized in our dataset as follows: 212464 frames as training set organized in sequences of variable length, 6000 frames as validation set organized in sequences of 16 frames, and 6384 frames for test divided in sequences of 16 frames. Note that the original videos are in 1920x1080 resolution and 25fps, so the dataset can be automatically re-generated up to such resolution and framerate.

\subsection{Static Tennis dataset}
\label{sec:static_tennis_dataset}
We adopt the \emph{Tennis} dataset of \cite{menapace2021pvg} to compare with previous playable video generation methods. The dataset is composed of video sequences from 2 matches recorded in the same arena and features 4 players with similar appearance. A total of 40 minutes of training videos is present. The validation and the test set are composed respectively of 2800 and 3280 frames divided in sequences of 16 frames acquired at 5fps. In order to satisfy the assumptions of previous methods, the dataset features limited camera movement and each video is cropped to depict only a single player in the lower part of the field.

%\vlad{The Datasets description can be significantly compressed.} 
%\noindent\textbf{Datasets.} We evaluate our method on four video datasets:\\
%\noindent \textbullet~\textit{Minecraft} dataset. We collect a synthetic video dataset with duration of 1h where two \emph{Minecraft} players perform a sparring session. The dataset features wide camera movement and diverse players. % to evaluate camera and style modeling capabilities.

%\noindent \textbullet~\textit{Minecraft Camera} dataset. We collect auxiliary \emph{Minecraft} sequences where the camera is moved in the neighborhood of a starting position. We use the frames obtained in this way as a convenient ground truth to evaluate camera manipulation capabilities.

%\noindent \textbullet~\textit{Tennis} dataset. We collect a large scale dataset of 43 tennis matches totalling 11.8h of videos. The dataset features different tennis fields and players to evaluate style modeling capabilities.

%\noindent \textbullet~\textit{Static Tennis} dataset. We adopt the \emph{Tennis} dataset of \cite{menapace2021pvg} to allow comparison with playable video generation methods. Differently from our \emph{Tennis} dataset, to satisfy the assumptions of previous methods, the dataset features limited camera movement and each video is cropped to depict only a single player.

%The dataset are further detailed in the \emph{Supp. Mat.}.
