# Supplementary material for: Playable Environments: Video Manipulation in Space and Time
Source: arXiv:2203.01914 source file (2022-03-15)
Supplement: Supplementary file 2 [file supplementary_experiments.tex]

\section{Experiments}
\label{sec:experiments}

In this section we show additional experimental results. Our experiments are complemented by a website (see \href{\webpage}{\webpagename}) showing additional video qualitative results including video sequences produced interactively by users,  camera and style manipulation results, and samples of dataset sequences. Sec.~\ref{sec:synthesis_module_user_study} shows a user study for the evaluation of video quality, Sec.~\ref{sec:playability_evaluation} shows additional playability evaluation results, Sec.~\ref{sec:playability_user_study} describes the user study for the evaluation of playability, Sec.~\ref{sec:synthesis_ablation_evaluation} shows ablation results for the synthesis module, Sec.~\ref{sec:action_ablation_evaluation} shows ablation results for the action module, Sec.~\ref{sec:camera_manipulation_evaluation} presents additional results for camera manipulation and Sec.~\ref{sec:style_manipulation_evaluation} shows style manipulation results.

\subsection{Synthesis module User Study}
\label{sec:synthesis_module_user_study}

In order to further evaluate video quality improvements with respect to CADDY \cite{menapace2021pvg}, we run a user study on video quality against \cite{menapace2021pvg} on the \emph{Static Tennis} dataset, the original dataset of \cite{menapace2021pvg}. Note that, for fairness of comparison, we make use of the \emph{Static Tennis} dataset which does not feature the several challenges addressed by our method but not by CADDY \cite{menapace2021pvg}, such as wide camera movements, multiple players and changes in appearance.

We create 206 video pairs with the two methods and ask 3 distinct AMT users to express their preference in terms of video quality between the two videos. 618 votes expressed by 18 distinct AMT users are gathered and assign a preference of 81.6\% to our method.

\subsection{Playability evaluation}
\label{sec:playability_evaluation}
\begin{table}
\begin{center}

\setlength{\tabcolsep}{1.0pt}
\footnotesize
\begin{tabular}{lccccccccccc}
\toprule
 & \emph{Aux.} & \emph{H.Res.} & $\mathcal{L}_{\Delta}$ & LPIPS$\downarrow$ & FID$\downarrow$ & FVD$\downarrow$ & $\Delta$-\emph{MSE}$\downarrow$ & $\Delta$-\emph{Acc}$\uparrow$ & ADD$\downarrow$ & MDR$\downarrow$\\
\midrule
(i) &&&& 0.743 & 288 & 3667 & 1.0 & (100) & \textbf{15.1} & 96.8 \\
(ii) &\checkmark&&& 0.773 & 296 & 2906 & 0.999 & 52.8 &  56.3 & 93.2 \\
(iii) &\checkmark&\checkmark&& 0.677 & 211 & 2213 & 0.998 & 53.7 & 42.5 & 82.9 \\
(iv) &\checkmark&&\checkmark& 0.707 & 275 & 2553 & 0.467 & \textbf{83.3}  & 56.2 & 92.2 \\
(v) &\checkmark&\checkmark&\checkmark& 0.691 & 309 & 2187 & 0.439 & 82.6 & 17.4 & 95.1 \\

\midrule

(Ours) &&&& \textbf{0.204} & \textbf{16.8} & \textbf{329} & \textbf{0.271} & 77.7 & 17.8 & \textbf{33.9} \\

\bottomrule
\end{tabular}
\end{center}
\caption{Comparison with baselines on the \textit{Minecraft} dataset. \emph{Aux.}: use of auxiliary bounding box and camera pose information; \emph{H.Res.} use of the high resolution model; $\mathcal{L}_{\Delta}$ use of the loss for $\Delta$-\emph{MSE}. $\Delta$-\emph{MSE}, $\Delta$-\emph{Acc} and MDR in \%, ADD in pixels.}
%\vspace{-1mm}
\label{table:playability_minecraft}
\end{table}

In Tab.~\ref{table:playability_minecraft}, we present playability evaluation results on the \emph{Minecraft} dataset. As for the \emph{Tennis} dataset, our method surpasses the baselines both in terms of video and action quality metrics. In particular, the high variation in camera pose in this dataset is not correctly modeled by the baseline methods which produce irrealistic results. Note that (i) and (iv) show a better $\Delta$-\textit{ACC} than our method which is explained by their learned action space which only discovers a reduced number of action categories as confirmed by the high $\Delta$-\textit{MSE} and by Fig.~\ref{fig:qualitatives_actions}.

We show qualitatives results for both the \emph{Minecraft} and \emph{Tennis} datasets in Fig.~\ref{fig:qualitatives_playability_reconstruction_minecraft} and Fig.~\ref{fig:qualitatives_playability_reconstruction_tennis} respectively. The movements of the players reconstructed by our method match the ones in the ground truth sequence, indicating that a good action representation is learned. In addition, our model synthesizes players performing motions that are more realistic than the ones produced by the baselines.

We show a representation of the learned action space on both the \emph{Minecraft} and \emph{Tennis} datasets in Fig.~\ref{fig:qualitatives_actions}.

\subsection{Playability User Study}
\label{sec:playability_user_study}
To further evaluate the quality of the action space we perform a user study (see Tab.~\ref{table:playability_user_study_tennis_reduced}) on the \emph{Tennis} dataset, following the protocol of \emph{Menapace} \etal~\cite{menapace2021pvg}. We sample a set of 26 frames from the test set and for each frame we produce video continuations conditioned on each learned action. Two separate videos are produced for each initial frame and action, the first cropped on the lower tennis field, the second cropped on the upper tennis field to ensure a single tennis player is depicted in each video. For each produces sequence, we ask 3 \emph{Amazon Mechanical Turk} users to choose which is the performed action between a set of options. We then measure agreement between the users using the Fleiss' kappa measure \cite{fleiss1971measuring} and compute diversity in the generated actions using entropy of user-selected actions. We consider only the baselines with the highest video quality and with the best action space metrics. Our model achieves the best agreement and comparable diversity to the baselines indicating that the model generates videos that are consistently conditioned by the action and that no mode collapse of the learned actions is present.

\begin{table}
\begin{center}

\setlength{\tabcolsep}{2.0pt}
\footnotesize
\begin{tabular}{lcccccccc}
\toprule
 & \emph{Aux.} & \emph{H.Res.} & $\mathcal{L}_{\Delta}$ & Agreement$\uparrow$ & Diversity$\uparrow$ & \emph{Other} votes\\
\midrule
CADDY \cite{menapace2021pvg} (iii) &\checkmark&\checkmark&& 0.353 & \textbf{1.77} & 1.86 \\
CADDY \cite{menapace2021pvg} (v)  &\checkmark&\checkmark&\checkmark& 0.170 & 1.71 & 24.7 \\

\midrule

(Ours) &&&& \textbf{0.444} & 1.7 & 0.80 \\

\bottomrule
\end{tabular}
\end{center}
\vspace{-8pt}
\caption{User study results on the \textit{Tennis} dataset. \emph{Aux.}: use of bounding boxes and camera pose; \emph{H.Res.} use of the high resolution model; $\mathcal{L}_{\Delta}$ use of the loss for $\Delta$-\emph{MSE}. \emph{Other} votes in \%.} 
%\vspace{-3mm}
\label{table:playability_user_study_tennis_reduced}
\end{table}

\subsection{Synthesis module Ablation Study}
\label{sec:synthesis_ablation_evaluation}

We present ablation study results for the synthesis module on the \emph{Tennis} dataset in Tab.~\ref{table:ablation_reconstruction_tennis_reduced} and present qualitative results in Fig.~\ref{fig:qualitatives_reconstruction_minecraft} and Fig.~\ref{fig:qualitatives_reconstruction_tennis} respectively for the \emph{Minecraft} and \emph{Tennis} datasets. The evaluation confirms the importance of the use of style modulation layers to model appearance changes and of the bending network to model deformations. In addition, without our feature renderer $F$, the model produces blurry results and lacks details such as the wrinkles on the clothes. Introducing the feature renderer $F$ allows the model to be trained on complete patches applying the perceptual loss term. This, in conjunction with the ability of ConvNets to model inter-pixel relationships, enables the model to reduce blur and to generate clothing that contains more detailed wrinkles. We also note that, in some sequences, the feature renderer is capable of generating realistic player shadows in portions of the image that lie outside of the bounding volume $\beta$ for the radiance field of the player. We ascribe this to the capacity of the ConvNet $F$ to model the correlation between the presence of the player and of its shadow.

\begin{table}
\begin{center}
\setlength{\tabcolsep}{1.8pt}
\footnotesize
\begin{tabular}{lccccccccc}
\midrule
Var. & \emph{Multi}\,$\langle$\textbf{3}$\rangle$ & $\pi$\,$\langle$\textbf{4}$\rangle$ & $w$\,$\langle$\textbf{5}$\rangle$ & $F$\,$\langle$\textbf{6}$\rangle$ & LPIPS$\downarrow$ & FID$\downarrow$ & FVD$\downarrow$  & ADD$\downarrow$ & MDR$\downarrow$ \\
\midrule
(a) &&&&& 0.505 & 256.1 & 7011 & 72.2 & 85.6 \\
(b) &\checkmark&&&& 0.619 & 271.4 & 10697 & 3.57 & 100.0 \\
(c) &\checkmark&\checkmark&&& 0.624 & 253.5 & 7280 & 2.65 & 28.6 \\
(d) &\checkmark&\checkmark&$\sim$&& 0.319 & 96.3 & 3303 & 79.8 & 85.4  \\
(e) &\checkmark&\checkmark&\checkmark&& 0.286 & 39.3 & 638 & 3.11 & 7.34 \\
(f) &\checkmark&\checkmark&\checkmark&$\sim$& 0.272 & 39.2 & 2678 & 46.9 & 60.5 \\
\midrule

Full &\checkmark&\checkmark&\checkmark&\checkmark& \textbf{0.167} & \textbf{17.1} & \textbf{497} & \textbf{2.56} & \textbf{3.90} \\
\midrule
\end{tabular}
\end{center}
\caption{Synthesis module ablation results on the \textit{Tennis} dataset. \emph{Multi}: use of multi-object modeling, $\pi$: use of deformation, $w$: use of style modulation layers or of direct style encoding ($\sim$), $F$: use of the feature renderer or of the simplified renderer ($\sim$). ADD in pixels, MDR in \%.}

\label{table:ablation_reconstruction_tennis_reduced}
\end{table}

\begin{figure}
     \centering

     \includegraphics[width=1.0\linewidth]{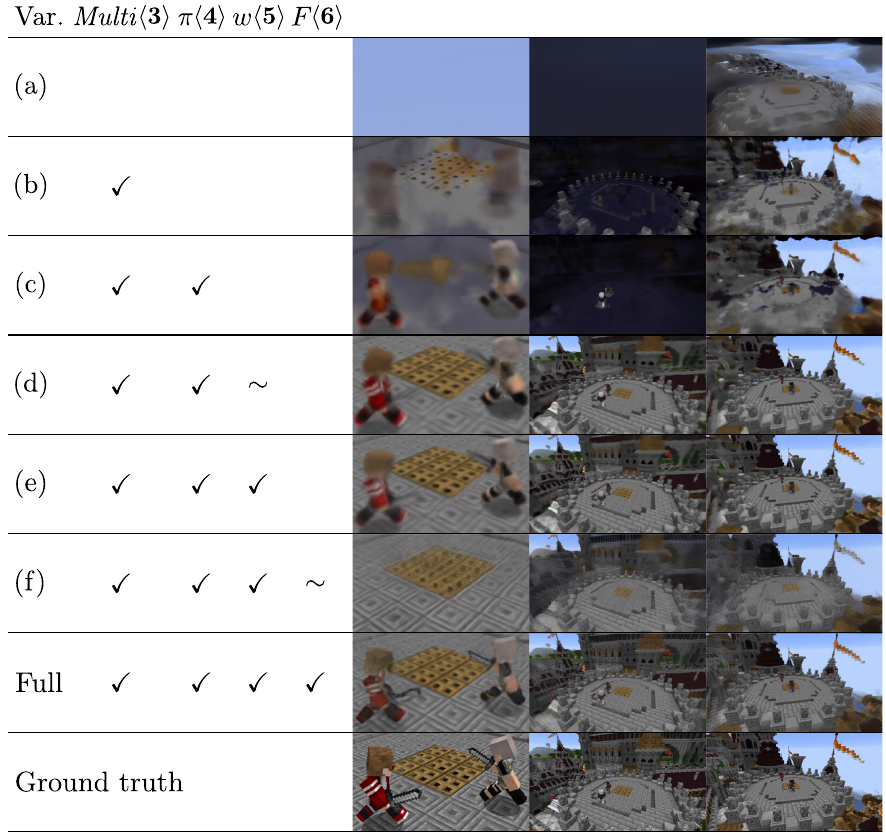}
     \caption{Synthesis module reconstruction results on the \emph{Minecraft} dataset. The first image is cropped for better visualization. \emph{Multi}: use of multi-object modeling, $\pi$: use of deformation, $w$: use of style modulation layers or of direct style encoding ($\sim$), $F$: use of the feature renderer or of the simplified renderer ($\sim$).}

    \label{fig:qualitatives_reconstruction_minecraft}
\end{figure}

\begin{figure}
     \centering

     \includegraphics[width=1.0\linewidth]{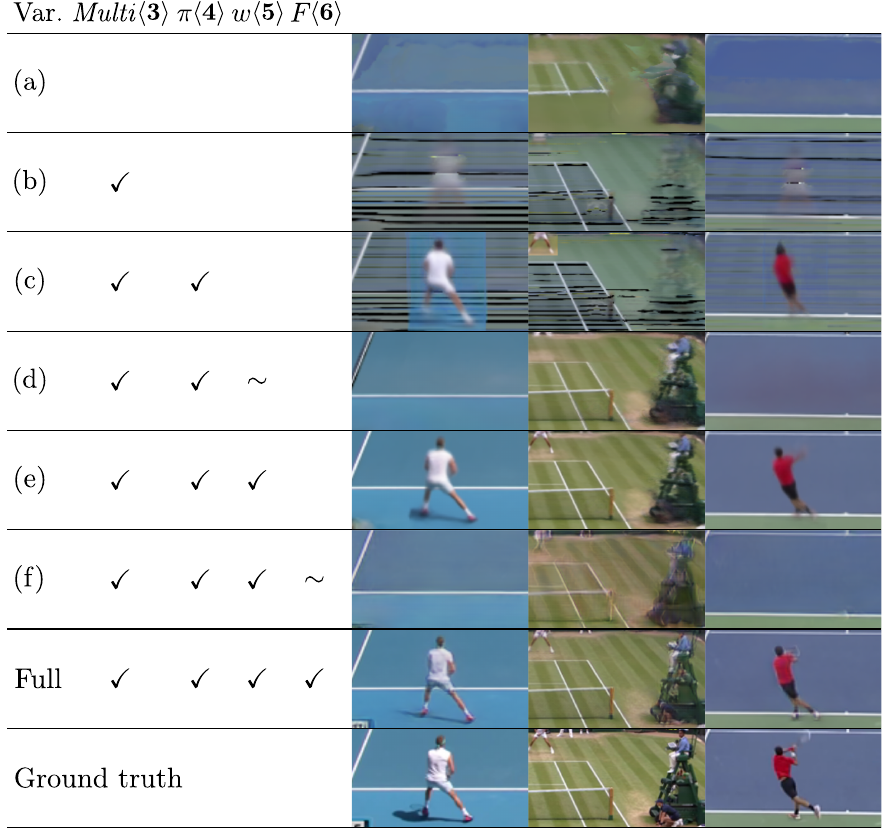}
     \caption{Synthesis module reconstruction results on the \emph{Tennis} dataset. The image is cropped for better visualization. \emph{Multi}: use of multi-object modeling, $\pi$: use of deformation, $w$: use of style modulation layers or of direct style encoding ($\sim$), $F$: use of the feature renderer or of the simplified renderer ($\sim$).}

    \label{fig:qualitatives_reconstruction_tennis}
\end{figure}

\subsection{Action module Ablation Study}
\label{sec:action_ablation_evaluation}

In Fig.~\ref{fig:qualitatives_playability_ablation__minecraft} we show qualitative results for the action module ablation study on the \emph{Minecraft} dataset. We note that, while method variations that do not use the temporal discriminator $D$ produce player movements closer to the ground truth sequence, they tend to produce less realistic motions for the moving players.

\subsection{Camera manipulation evaluation}
\label{sec:camera_manipulation_evaluation}
\begin{table}
\begin{center}
\setlength{\tabcolsep}{1.8pt}
\footnotesize
\begin{tabular}{lcccccccc}
\midrule
& \emph{Aux.} & \emph{H.Res.} & $\mathcal{L}_{\Delta}$ & LPIPS$\downarrow$ & FID$\downarrow$  & ADD$\downarrow$ & MDR$\downarrow$ \\
\midrule
(i) &&&& 0.659 & 224 & 50.4 & 82.0 \\
(ii) &\checkmark&&& 0.623 & 170 & 54.7 & 33.7 \\
(iii) &\checkmark&\checkmark&& 0.425 & 26.1 & 38.1 & 29.2 \\
(iv) &\checkmark&&\checkmark& 0.634 & 164 & 57.4 & 41.7 \\
(v) &\checkmark&\checkmark&\checkmark& 0.574 & 216 & 35.0 & 66.7 \\
\midrule
(Ours) &&&& \textbf{0.205} & \textbf{20.5} & \textbf{13.9}  & \textbf{5.76} \\
\midrule
\end{tabular}
\end{center}
\caption{Camera control evaluation results on the \textit{Tennis} dataset. \emph{Aux.}: use of bounding boxes and camera pose; \emph{H.Res.} use of the high resolution model; $\mathcal{L}_{\Delta}$ use of the loss for $\Delta$-\emph{MSE}. ADD in pixels, MDR in \%.}

\label{table:camera_manipulation_tennis_reduced}
\end{table}

We evaluate camera manipulation capabilities for our method on the \emph{Tennis} dataset. We consider each test sequence and sample two random camera poses by applying noise to the camera pose parameters in the first frame. We then generate a camera trajectory by interpolating between the two poses and render the sequence from the novel camera trajectory. Note that in the \emph{Tennis} dataset the largest portion of the image is occupied by the field plane. Consequently, we can approximately match each image rendered from the novel trajectory to the corresponding original image by applying a homography. We then compute reconstruction losses between the original and the generated sequence warped according to the corresponding homography. While this evaluation does not account for parts of the image that do not lie on the field plane such as the players, it can be used to detect failure cases. We show the results in Tab.~\ref{table:camera_manipulation_tennis_reduced}. LPIPS, ADD and MDR highlight that our method obtains better consistency than the baselines in the generation of novel camera views. In addition, we show qualitatives in Fig.~\ref{fig:qualitatives_camera_manipulation_minecraft} and Fig.~\ref{fig:qualitatives_camera_manipulation_tennis} respectively for the \emph{Minecraft} and \emph{Tennis} dataset.

\subsection{Style manipulation evaluation}
\label{sec:style_manipulation_evaluation}
In Fig.~\ref{fig:qualitatives_style_minecraft} and Fig.~\ref{fig:qualitatives_style_tennis} we show qualitative style manipulation results obtained with our method. We consider a target style image from which we extract the style code $w$ for each object. We then replace the style code in the environment state extracted from a source image with the target style and re-render the image using the synthesis module. Our method can successfully change the appearance of the players and of the static scene elements.

% TODO comment results for the camera manipulation task on Tennis

%We address this issue with an AMT user study where users are asked to express preference between two corresponding sequences generated from the novel trajectory by different methods. Each video is overlaid with the position that the field lines should occupy under the novel camera view and users are specifically asked to pay attention to whether the overlaid lines match the generated ones.

%\willi{Explain in which space the delta is computed for each dataset}
%\willi{Training of the rcnn on minecraft}

\begin{figure*}
    \centering
    \includegraphics[width=1.0\textwidth]{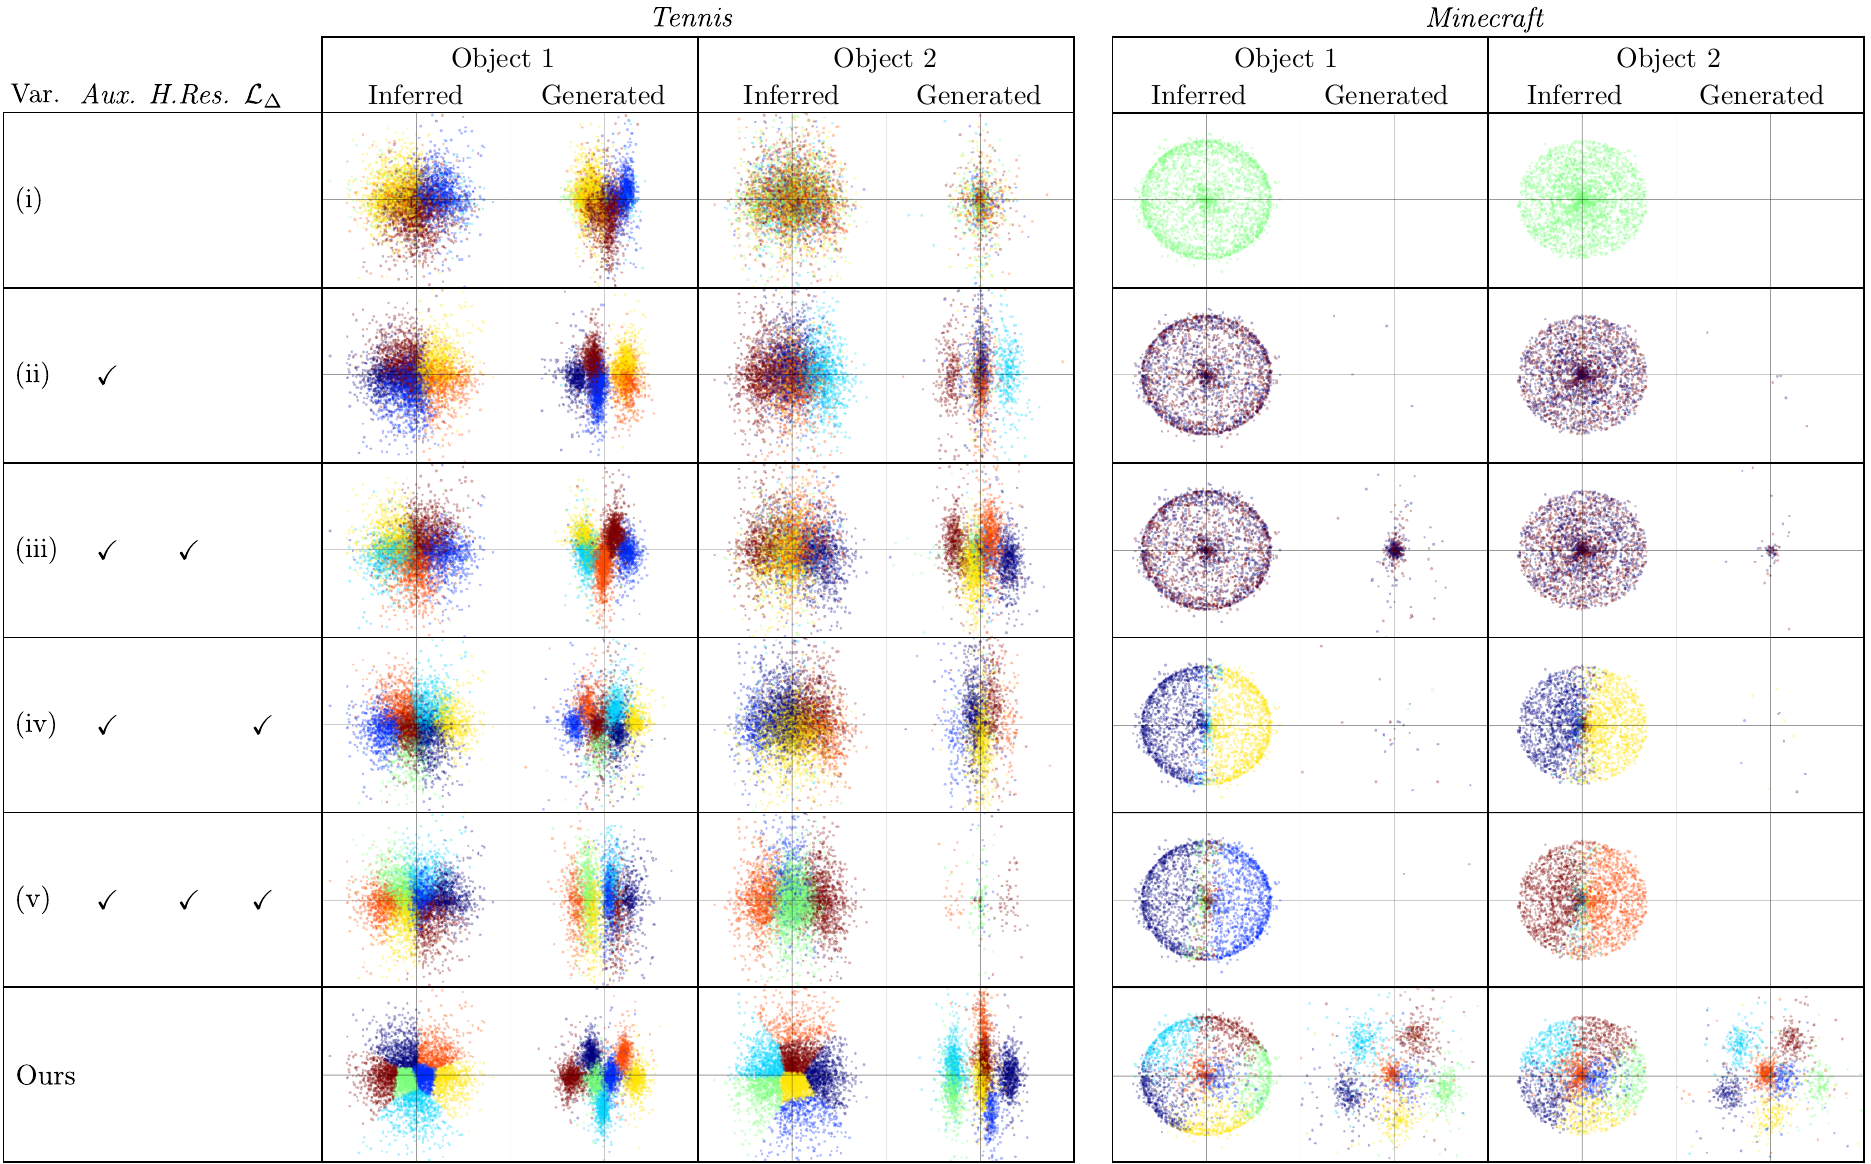}
    \caption{Visualization of the learned action space on the \emph{Minecraft} and \emph{Tennis} datasets for our method and the baselines. Each plot shows $\Delta$ movements of the playable objects measured on the ground plane between a pair of successive frames. Colors indicate the different action label that is associated to each movement. `Inferred' movements are measured on the test sequences, thus the plots shows the actions inferred by the action network as a function of the input states. `Generated' movements are measured on the generated sequences, thus the plots show the movement generated by the dynamics network as a response to the current action input. It can be observed that our method produces sharper decision boundaries between the actions associated to movement. In addition, the distribution of `Generated' movements produced as a response to each action input matches the distribution of the `Inferred' movements associated to the same action. \emph{Aux.}: use of auxiliary bounding box and camera pose information; \emph{H.Res.} use of the high resolution model; $\mathcal{L}_{\Delta}$ use of the loss for $\Delta$-\emph{MSE}.}
    \label{fig:qualitatives_actions}
\end{figure*}
\begin{figure*}
    \centering
    \includegraphics[width=1.0\textwidth]{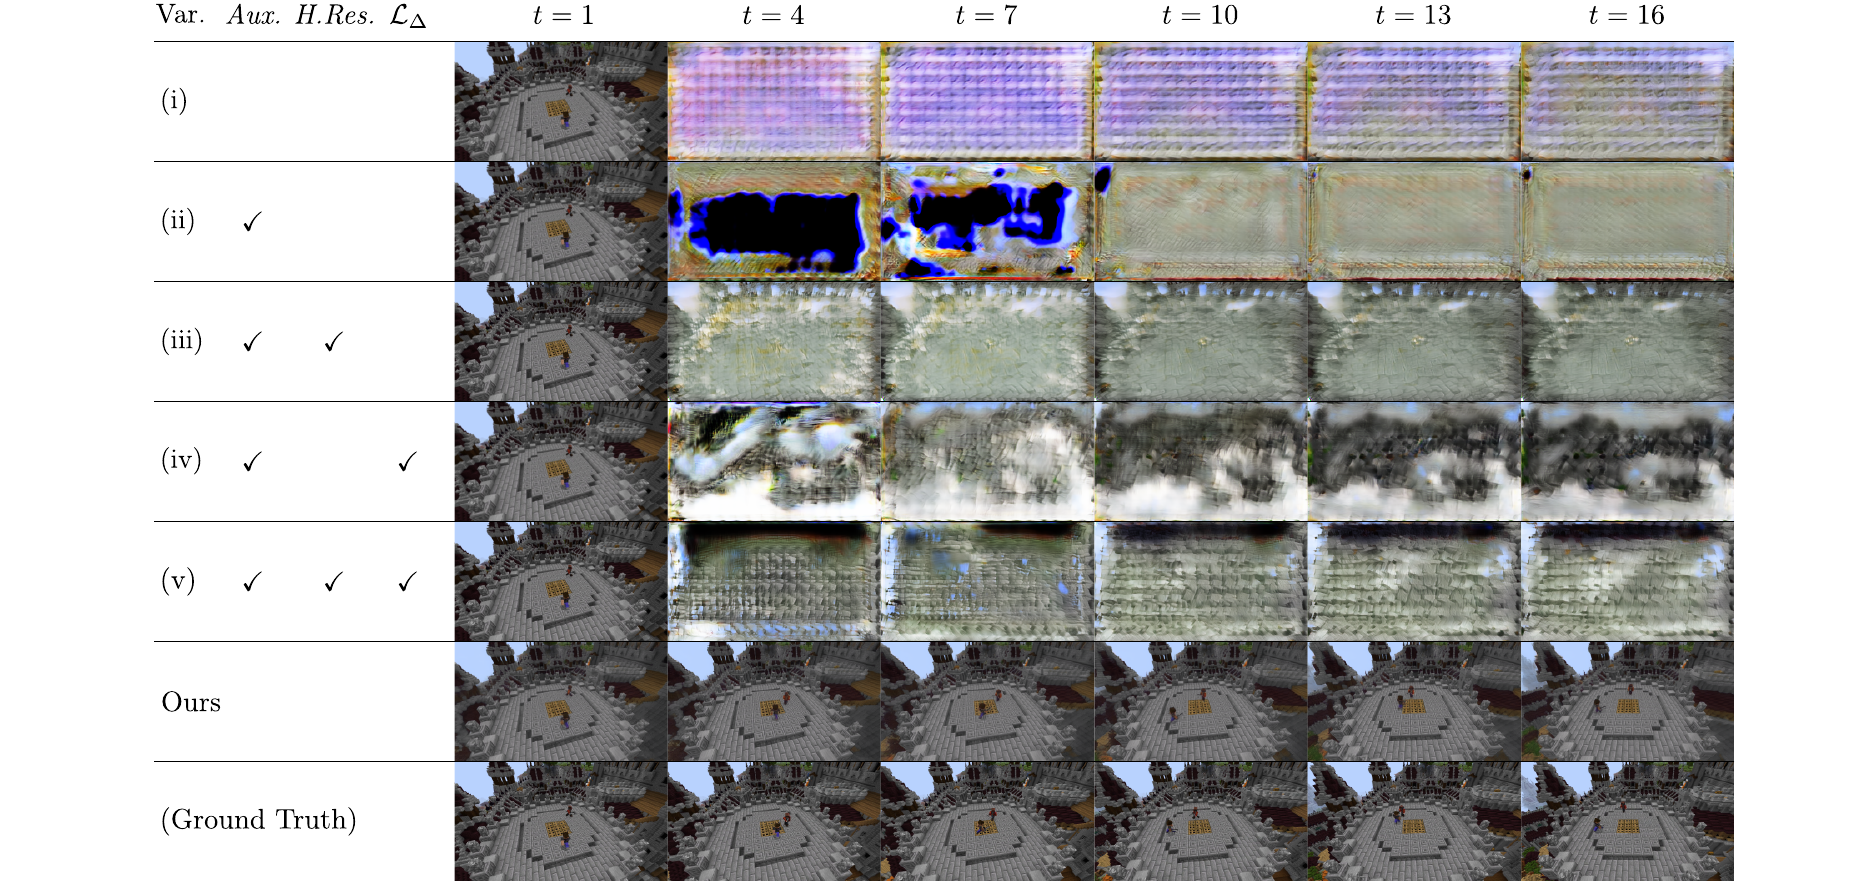}
    \caption{Reconstruction results on the \textit{Minecraft} dataset. Starting from the first frame, the dynamics network reconstructs the ground truth video using the sequence of discrete actions inferred by the action network on the original sequence. \emph{Aux.}: use of auxiliary bounding box and camera pose information; \emph{H.Res.} use of the high resolution model; $\mathcal{L}_{\Delta}$ use of the loss for $\Delta$-\emph{MSE}.}
    \label{fig:qualitatives_playability_reconstruction_minecraft}
\end{figure*}
\begin{figure*}
    \centering
    \includegraphics[width=1.0\textwidth]{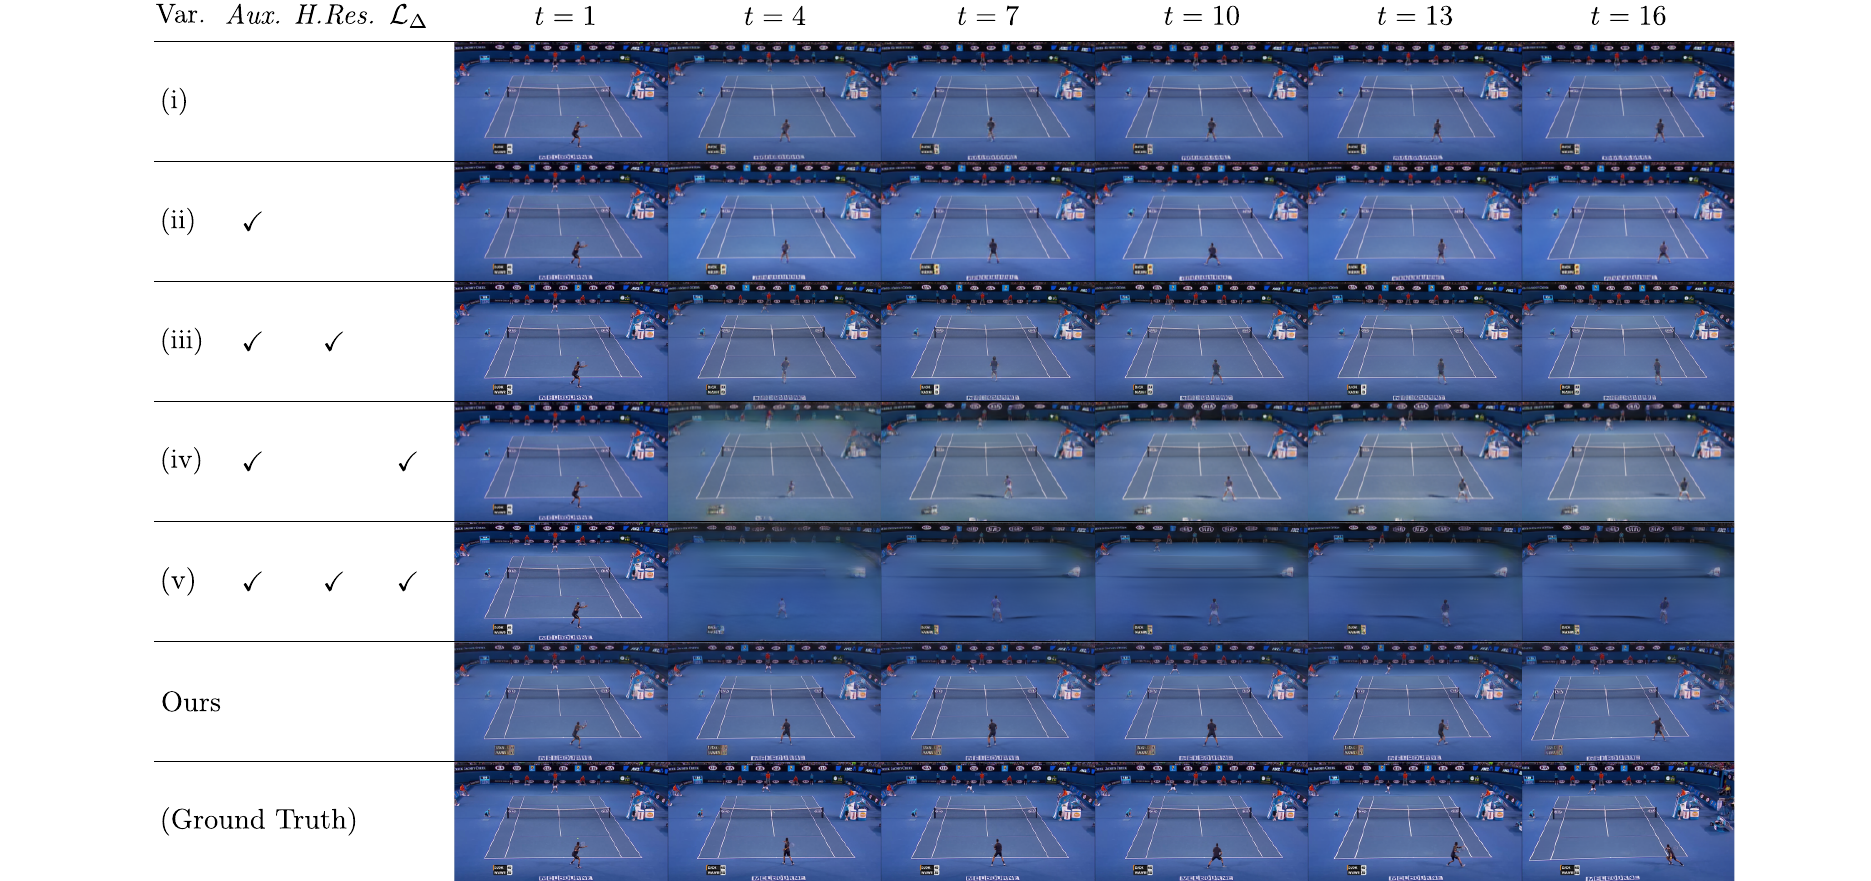}
    \caption{Reconstruction results on the \textit{Tennis} dataset. Starting from the first frame, the dynamics network reconstructs the ground truth video using the sequence of discrete actions inferred by the action network on the original sequence. \emph{Aux.}: use of auxiliary bounding box and camera pose information; \emph{H.Res.} use of the high resolution model; $\mathcal{L}_{\Delta}$ use of the loss for $\Delta$-\emph{MSE}.}
    \vspace{2cm}
    \label{fig:qualitatives_playability_reconstruction_tennis}
\end{figure*}
\begin{figure*}
    \centering
    \includegraphics[width=1.0\textwidth]{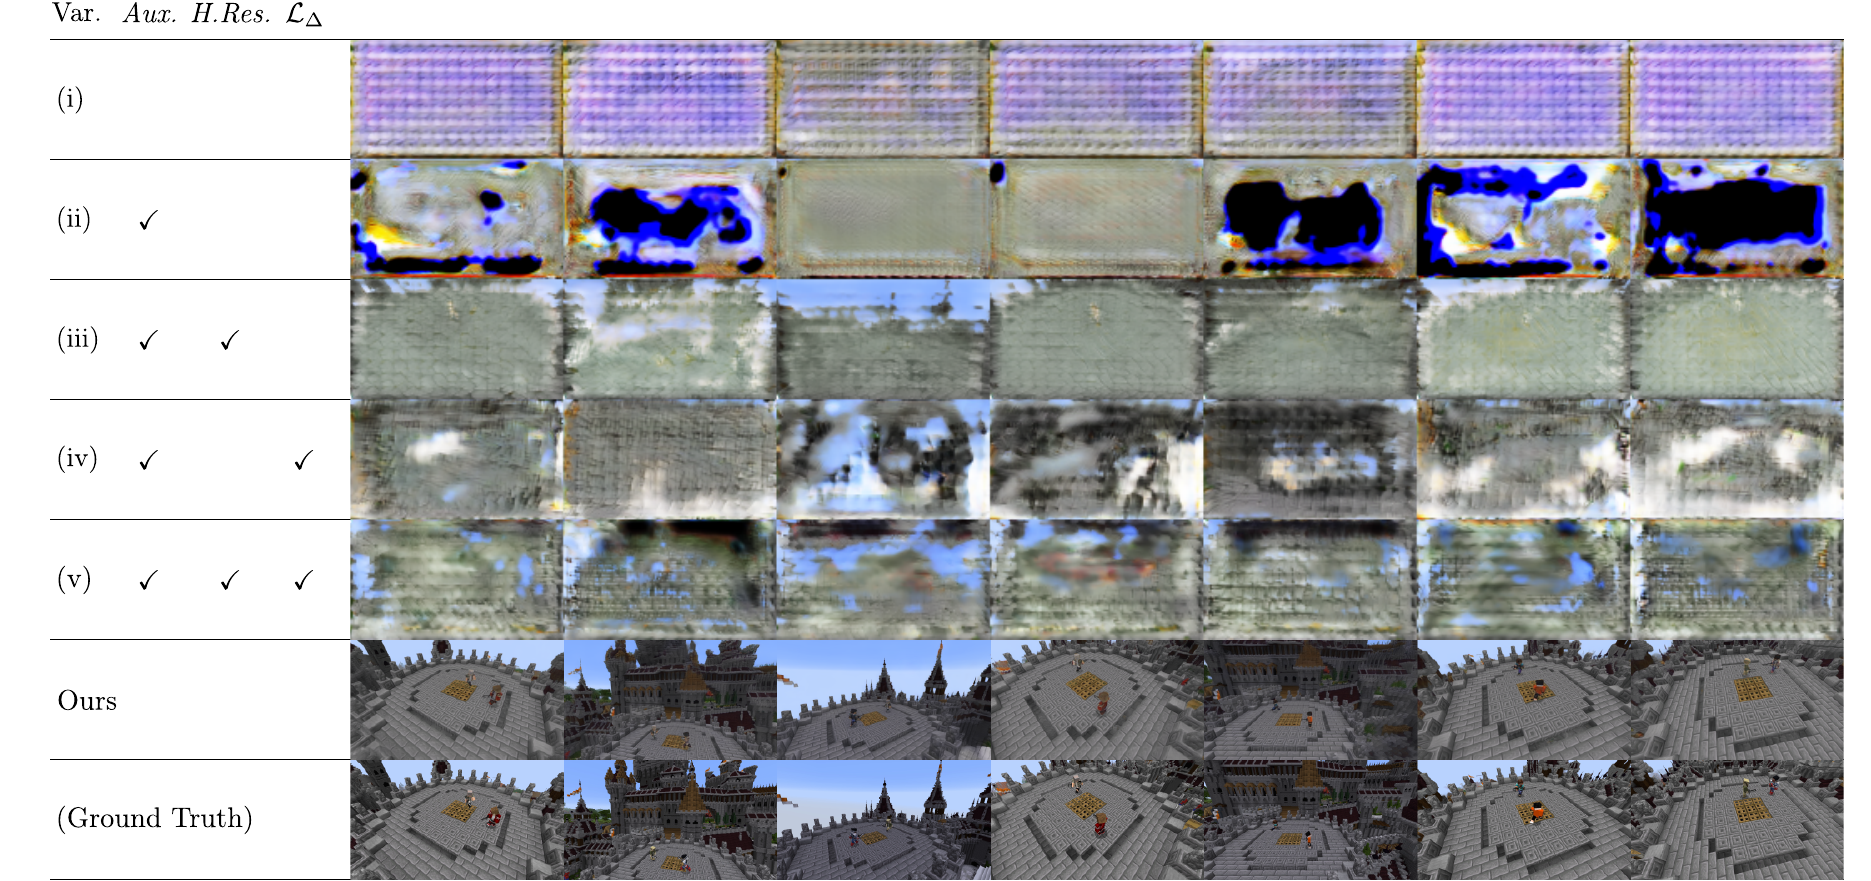}
    \caption{Camera manipulation results on the \textit{Minecraft Camera} dataset. Ground truth shows the reference frame, upper rows show camera manipulation results. \emph{Aux.}: use of auxiliary bounding box and camera pose information; \emph{H.Res.} use of the high resolution model; $\mathcal{L}_{\Delta}$ use of the loss for $\Delta$-\emph{MSE}.}
    \label{fig:qualitatives_camera_manipulation_minecraft}
\end{figure*}
\begin{figure*}
    \centering
    \includegraphics[width=1.0\textwidth]{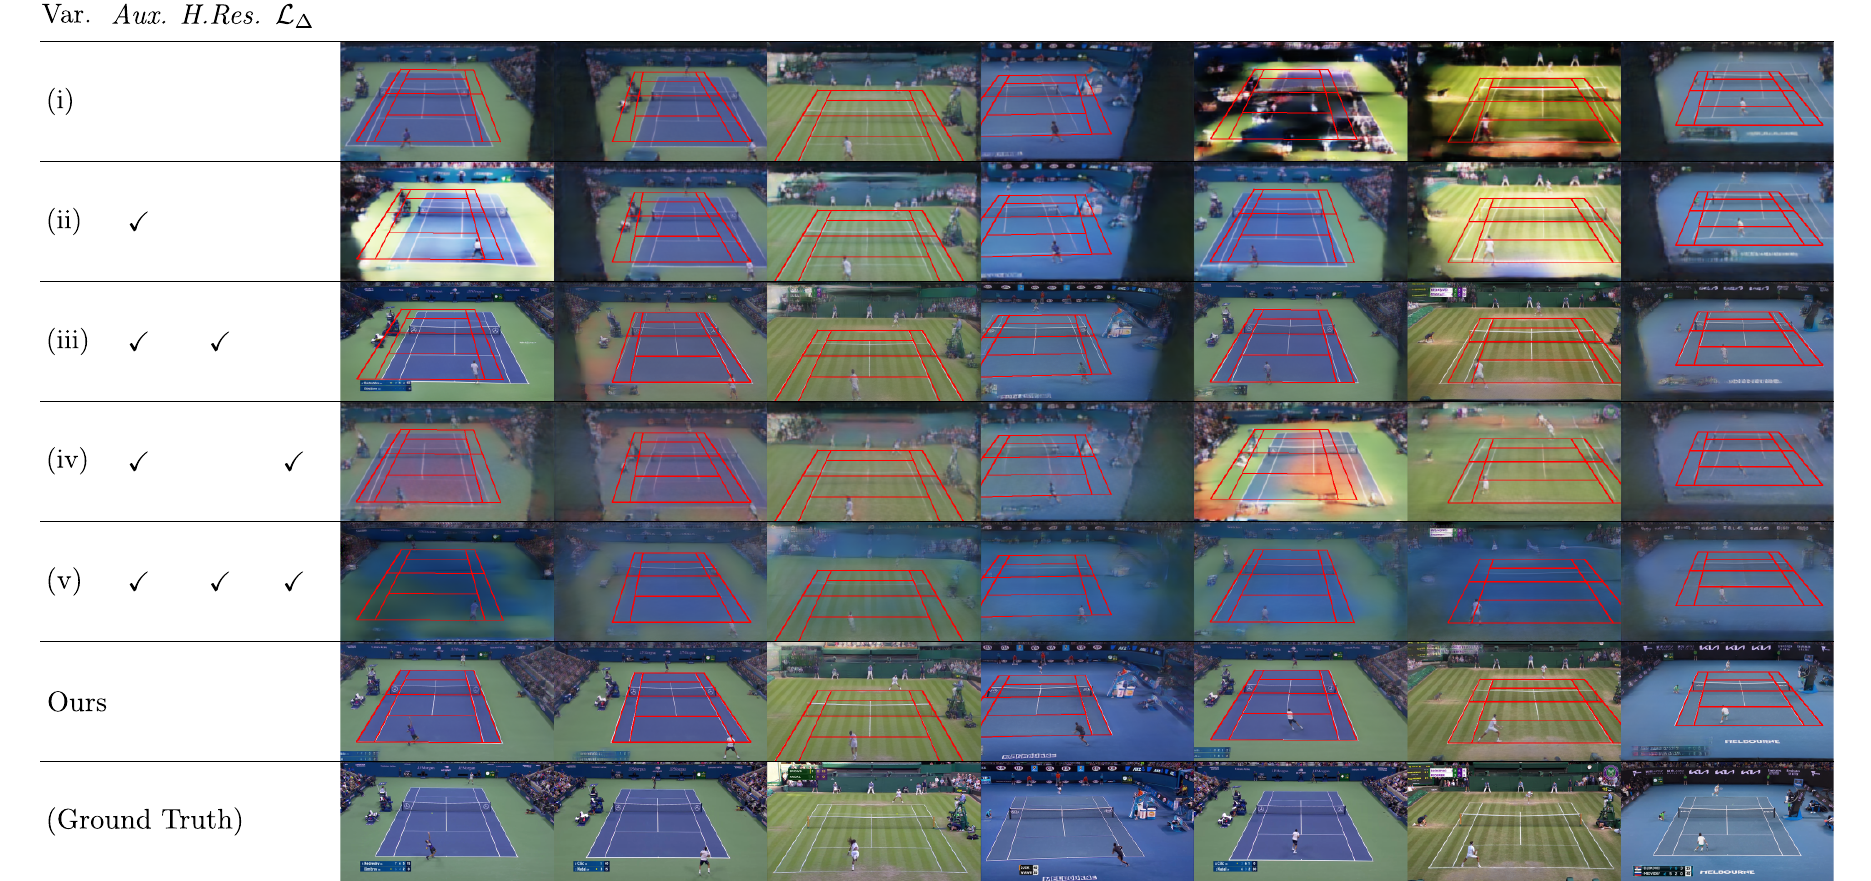}
    \caption{Camera manipulation results on the \textit{Tennis} dataset. Ground truth shows the reference frame, upper rows show camera manipulation results. To highlight camera manipulation errors, we overlay each generated image with the position where the field lines should be synthesized under the manipulated camera pose. \emph{Aux.}: use of auxiliary bounding box and camera pose information; \emph{H.Res.} use of the high resolution model; $\mathcal{L}_{\Delta}$ use of the loss for $\Delta$-\emph{MSE}.}
    \vspace{1cm}
    \label{fig:qualitatives_camera_manipulation_tennis}
\end{figure*}

\begin{figure*}
    \centering
    \includegraphics[width=1.0\textwidth]{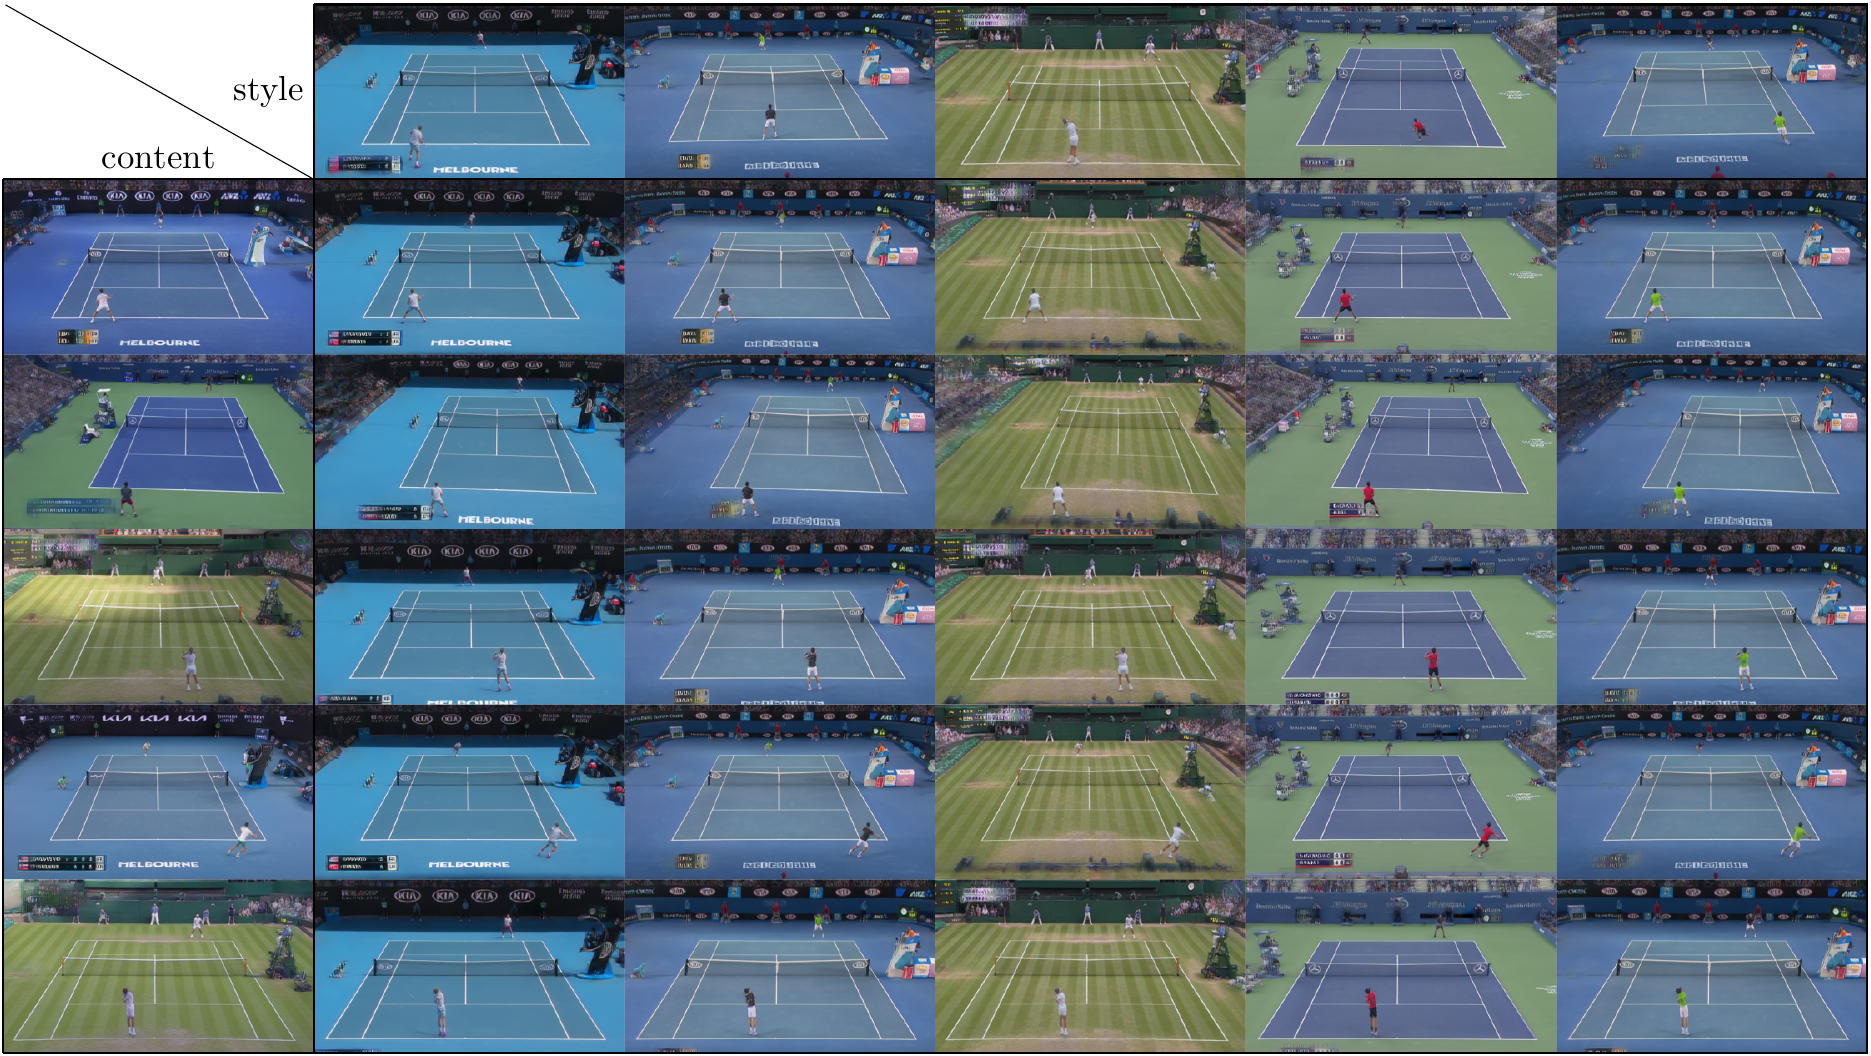}
    \caption{Style transfer results on the \textit{Tennis} dataset. The topmost row shows the target style, the leftmost column shows the image in which the style is injected.}
    \label{fig:qualitatives_style_tennis}
\end{figure*}
\begin{figure*}
    \centering
    \includegraphics[width=1.0\textwidth]{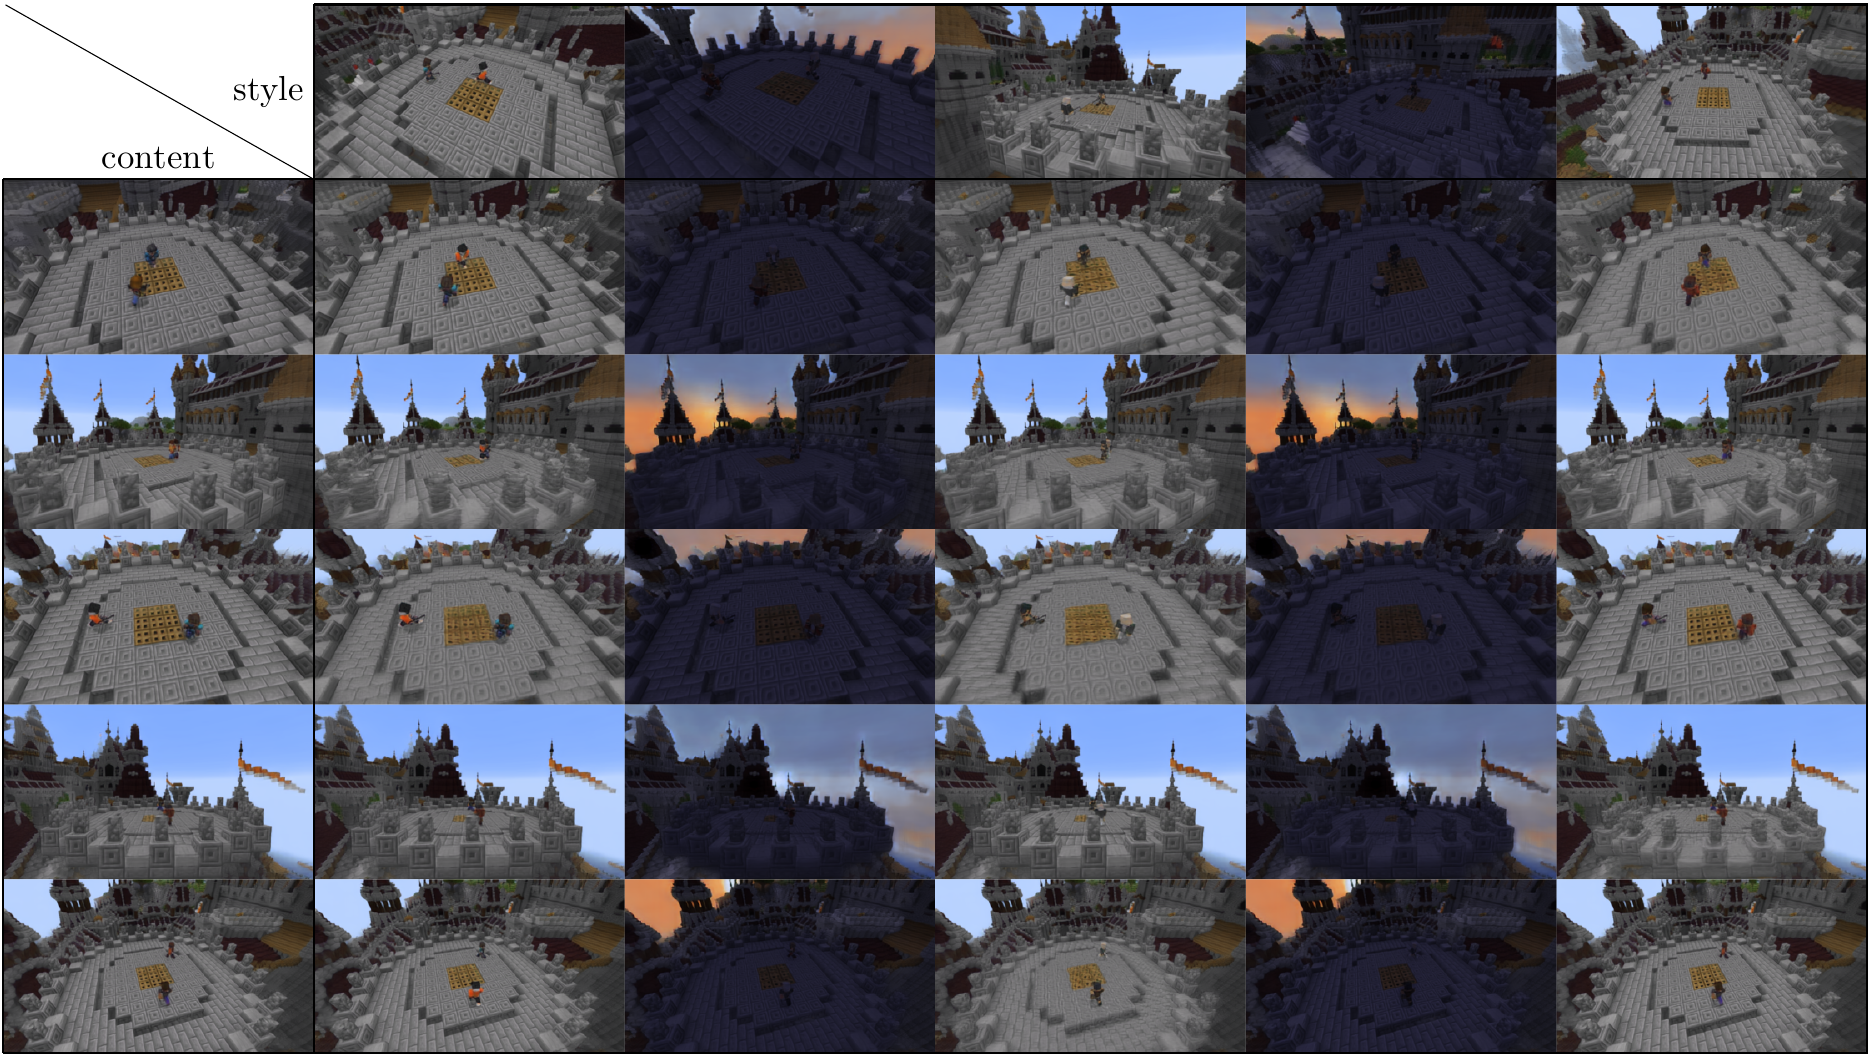}
    \caption{Style transfer results on the \textit{Minecraft} dataset. The topmost row shows the target style, the leftmost column shows the image in which the style is injected.}
    \label{fig:qualitatives_style_minecraft}
\end{figure*}

\begin{figure*}
    \centering
    \includegraphics[width=1.0\textwidth]{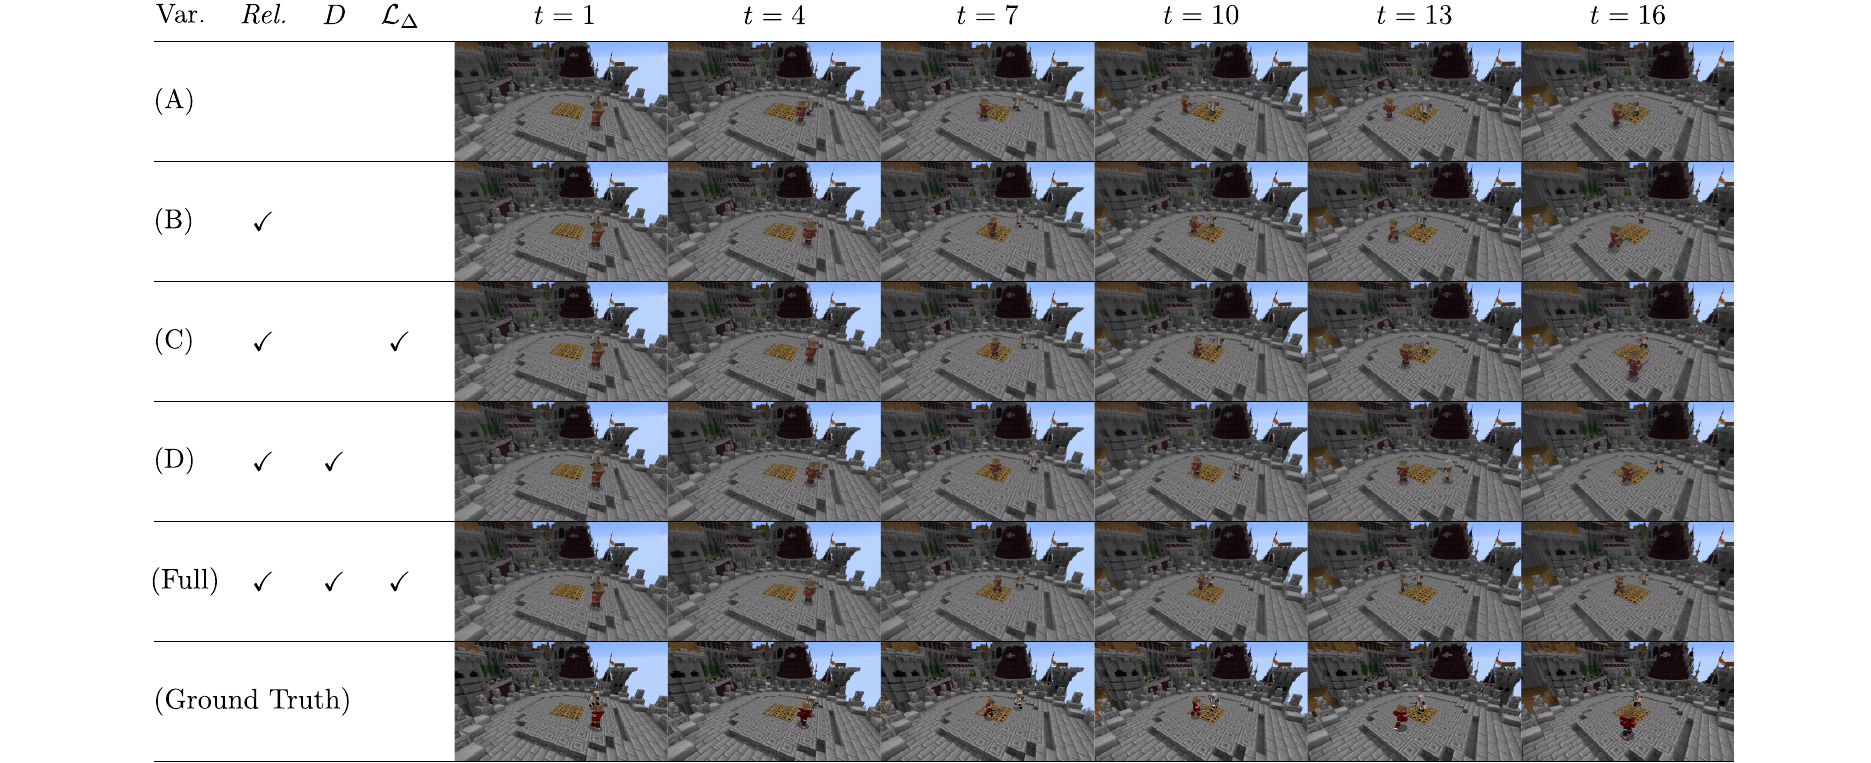}
    \caption{Reconstruction results on the \textit{Minecraft} dataset. Starting from the first frame, the dynamics network reconstructs the ground truth video using the sequence of discrete actions inferred by the action network on the original sequence. \emph{Rel.} use of camera relative residual $\Delta$ output, $D$ use of the temporal discriminator, $\mathcal{L}_{\Delta}$: use of the loss for $\Delta$-\emph{MSE}.}
    \label{fig:qualitatives_playability_ablation__minecraft}
\end{figure*}
