# Supplementary material for: Playable Environments: Video Manipulation in Space and Time
Source: arXiv:2203.01914 source file (2022-03-15)
Supplement: Supplementary file 3 [file supplementary_limitations.tex]

\section{Discussion}
\label{sec:discussion}
The following section discusses the main limitations of the method and social implications.

\noindent\textbf{Limitations.}  Our method performs some assumptions on the structure of the environment. First, while the appearance of the environment can change, the method assumes a constant geometry of the environment, preventing it from operating on datasets with actions performed in environments with different geometries. Second, in order to estimate the pose of dynamic objects, the method assumes that moving objects are located on the $y=0$ plane. Lastly, while on the \emph{Minecraft} dataset our method is learns a full 3D environment, on the \emph{Tennis} dataset the presence of camera rotations but not of camera translations makes the problem of recovering the field geometry ill-posed. We thus impose a ``flat world'' prior in order to regularize the geometry learned on this dataset, which is detailed in Sec.~\ref{sec:object_configurations}. This prior allows wider camera manipulations at inference time, but has the effect of projecting parts of the background on flat surfaces, causing visual artifacts when the position of the camera differs from the one of the original dataset.

We also note that our method exhibits blur artifacts or missing-part artifacts in regions of the scene corresponding to thin and fast-moving objects such as the limbs of players or the rackets. The challenging nature of the \emph{Tennis} dataset with frequent motion blur, object parts as small as a few pixels (eg. limbs) and noise in camera calibration is the main reason behind these artifacts that are partially addressed by our feature renderer.

When learning actions, it is important to consider both ease of manipulation, and the portion of interesting actions that can be captured. Users are typically mainly interested in manipulating the position of objects which is often correlated to the change in poses. Thus, to ease the manipulation, we found an ideal solution in learning actions related to changes in position and letting the  model  synthesize the corresponding change in poses. The main limitation caused by this tradeoff between action space simplicity and action space expressiveness is that it is difficult to control the synthesis of actions featuring changes in pose that are not directly correlated to changes in position, such as the swing of the racket.

Lastly, we remark that at inference time objects in the scene are animated independently from each other. This can generate artifacts such as both tennis players swinging the rackets at the same time and makes it not possible to capture interactions between objects in the scene.

\noindent\textbf{Social Implications.}  Similarly to methods operating on face and human appearances, our method could be used to deceive, and can potentially be used to tamper video sequences for nefarious purposes. However, we note that the constant environment geometry assumed by the method provides some protection against fraudulent uses since the method requires a certain scene to appear in many videos in the training dataset in order to allow its subsequent manipulation. This would make it not straightforward to tamper an isolated video for which the malicious individual does not dispose of a corresponding collection of videos of the same scene to use for training. We believe that the benefits brought in terms of novel creative applications and enhancements to user creativity outweigh the potential risks.

\begin{comment}
\noindent\textbf{Limitations.} 
% 
Our method % is limited by the 
assumes constant geometry of the environment, preventing it from operating on datasets with actions in different environments. In addition, on the \emph{Tennis} dataset the presence of camera rotations but not of camera translations makes the problem of recovering the field geometry ill-posed and a ``flat world'' assumption is necessary for this dataset (see \emph{Supp. Mat.}).
% 
% In addition, our method performs optimally when actions are linked to movement of the playable objects and has reduced performance in the identification of actions related to change in pose. 
Next, the performance drops when identifying actions related to change in pose. 
% 
% We ascribe this behavior to the increased complexity of actions expressed in the space of poses. 
% 

\noindent\textbf{Social Implications.} 
% 
While, similarly to methods operating on face and human appearances, our method could be used to deceive, we believe that the benefits brought in terms of novel creative applications outweigh the potential risks.
%Though not negligible, the impact of potential misuses of our method is low compared to that of methods operating on face and human appearances.
\end{comment}
