# Supplementary material for: Playable Environments: Video Manipulation in Space and Time
Source: arXiv:2203.01914 source file (2022-03-15)
Supplement: Supplementary file 4 [file supplementary_method.tex]

\section{Implementation Details}
\label{sec:implementation}

In this section, we discuss additional implementation details for our method. Sec.~\ref{sec:intro_nerf} introduces NeRF \cite{mildenhall2020nerf}, Sec.~\ref{sec:architecture_details} discusses the architecture of the models adopted in our method, Sec.~\ref{sec:feature_renderer} discusses the implementation details of our feature renderer ConvNet, Sec.~\ref{sec:object_configurations} describes the organization of the objects of which the environment is composed, Sec.~\ref{sec:model_sharing} describes the sharing strategies that are used to model different instances of the same object class and Sec.~\ref{sec:masking} describes details regarding batch normalization and pooling operations in the action module.

\subsection{Introduction to NeRF}
\label{sec:intro_nerf}
NeRF \cite{mildenhall2020nerf} represents scenes as radiance fields: a 5D continuous function that maps a 3D position and a 2D viewing direction to an emitted color $c$ and an opacity $\sigma$. NeRF parametrizes such function as an MLP.

Given a desired camera perspective, the associated image can be rendered exploiting the radiance field representation \cite{mildenhall2020nerf}. A ray $r$ is traced through each pixel and the associated color is obtained by integration:
\begin{equation}
    C(r) = \int_{t_n}^{t_f} T(t)\sigma(r(t))c(r(t)) dt 
\end{equation}
with
\begin{equation}
    T(t) = \mathrm{exp}\left(-\int_{t_n}^{t} \sigma(r(s)) ds\right)
\end{equation}
where $T(t)$ denotes the accumulated transmittance, and $t_n$ and $t_f$ represent the minimum and maximum distance from the camera in which the integration is performed. In practice, the integral can be approximated through quadrature \cite{mildenhall2020nerf}. $N$ positions along each ray $r$ are sampled and the associated color is computed as
\begin{equation}
    \hat{C}(r) = \sum_{i=1}^{N} T_i (1 - e^{-\sigma_i\delta_i}) c_i
\end{equation}
with
\begin{equation}
    T_i = \mathrm{exp}({-\sum_{j=1}^{i-1} \sigma_j\delta_j})
\end{equation}
where $c$ and $\sigma$ are obtained by querying the MLP and $\delta$ denotes the distance between successive samples.

In order to ease the learning of high frequency details, NeRF employs positional encodings of the 3D position and viewing direction as input to the underlying MLP.
In addition, \emph{Mildenhall} \etal \cite{mildenhall2020nerf} propose a stratified sampling approach which exploits a \emph{coarse} neural radiance field to locate portions of the ray corresponding to visible surfaces and allocates additional samples to the neighborhood of such regions. A \emph{fine} neural radiance field is used to compute the final image using both the initial and the additional sampled locations.

The model is trained using L2 distance between the reconstructed and the ground truth color value for each sampled ray.

\begin{figure*}
    \centering
    \includegraphics[width=1.0\textwidth]{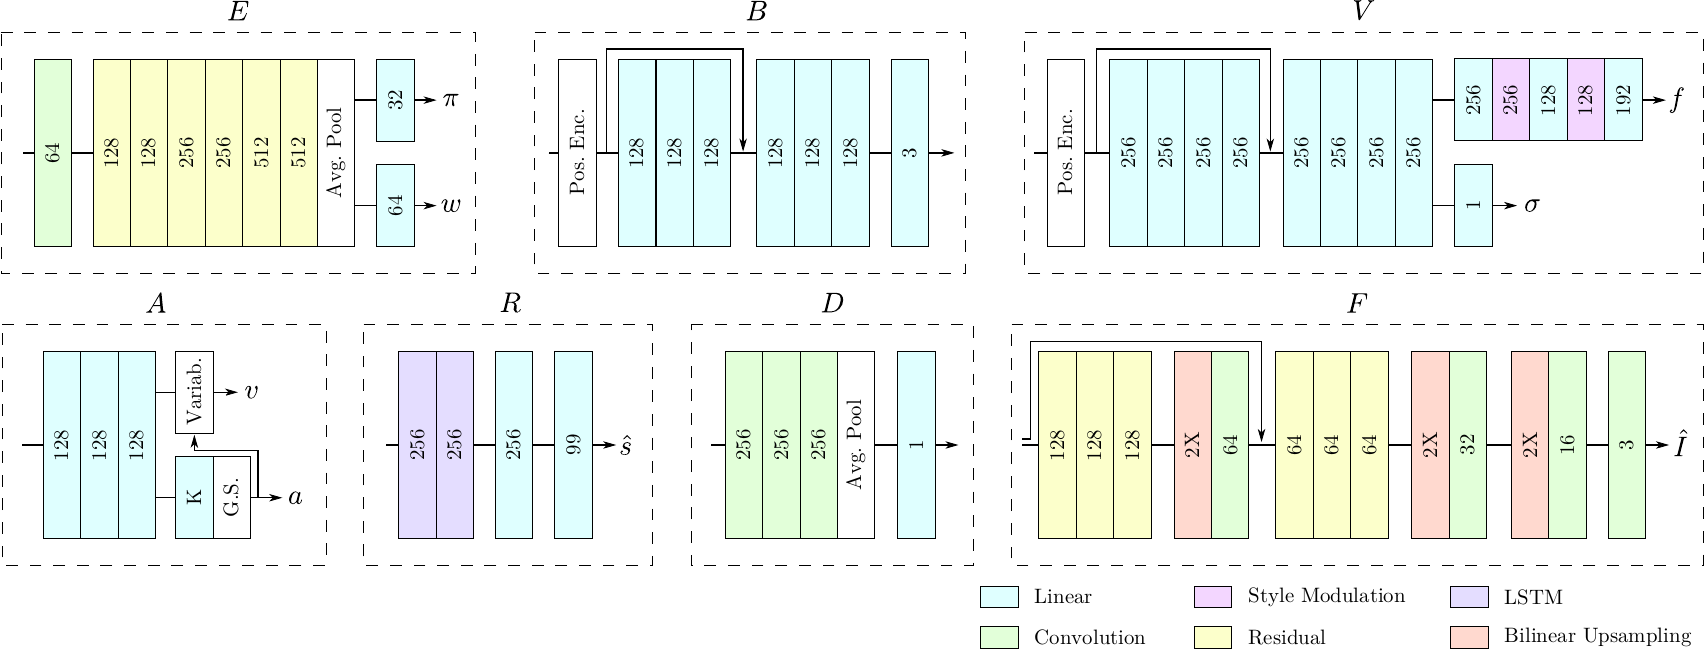}
    \caption{Architecture of the models employed by our method on the \emph{Tennis} dataset. The number in each block indicates the number of output features or the upsampling factor in the case of upsampling operations. Merging of arrows indicates concatenation. The architecture for the encoder $E$ refers to the encoder for the static object models. We adopt a smaller encoder for the players. \emph{G.S.} indicates Gumbel Softmax \cite{jang2017gumbel}; \emph{Pos. Enc.} indicates positional encoding.}
    \label{fig:architecture_details}
\end{figure*}
\subsection{Architecture details}
\label{sec:architecture_details}
In this section, we discuss the details of the models employed in our framework. Fig.~\ref{fig:architecture_details} shows the models employed on the \emph{Tennis} dataset.

We make use of positional encodings \cite{mildenhall2020nerf} for both $V$ and the bending network $B$. We use 10 and 6 octaves respectively and use the concatenation of the original vector and the encodings as input. Following \cite{park2021nerfies}, we gradually introduce the positional encodings in $B$ during the first 60.000 training iterations. No viewing direction is given as input to $B$ and $V$ to avoid artifacts when the environment is rendered from a camera pose outside of the training distribution. In addition, to reduce memory consumption, we do not make use of the hierarchical sampling scheme (see Sec.~\ref{sec:intro_nerf}).

We model the action network $A$ following \cite{menapace2021pvg} and make use of gumbel softmax sampling \cite{jang2017gumbel} to obtain discrete action representations. In addition, to foster $A$ in predicting actions that are associated to movement, we use only object positions $x_t$ as input rather than the complete environment state $s_t$.

The temporal discriminator $D$ receives as input the object positions $x$ and object poses $\pi$ and is further conditioned on the actions $a$ and action variabilities $v$ inferred on the ground truth sequence.

We modulate the number of residual blocks in $E$ based on the expected size of the input image crop.

\subsection{Feature Renderer Details}
\label{sec:feature_renderer}
We propose to render feature maps at multiple resolutions into the final image using a ConvNet feature renderer $F$. Our ConvNet accepts feature maps $\{f_i\}_{i=1}^{l}$ at $l$ different resolutions, each associated to a downsampling factor $d_i$. We obtain feature map $f_i$ by integration of the features sampled along the rays corresponding to pixel $I_{mn}$ in the original image, such that
\begin{equation}
\begin{gathered}
    m \in \left\{\frac{d_i}{2} + 1 + kd_i\right\}_{k=0}^{\frac{h}{d_i} - 1}, n \in \left\{\frac{d_i}{2} + 1 + kd_i\right\}_{k=0}^{\frac{w}{d_i} - 1}
\end{gathered}
\end{equation}
where $h$ and $w$ are the image height and width and indexes are expressed starting from 1. The process is illustrated in Fig.~\ref{fig:feature_renderer}. Note that each ray is sampled on a grid where the points are at a vertical and horizontal distance of $d_i$ from one another and at distance $d_i / 2$ from the border (see left of Fig.~\ref{fig:feature_renderer} for a visualization of the sampled positions). Note also that the ray is sampled at the pixel location in the original image that corresponds to the center of the associated local patch that will be synthesized by $F$.

In our implementation, we render two separate feature maps at downsampling factors 8x and 4x (see Fig.~\ref{fig:architecture_details}) to capture details at different scales. Note that this approach allows rendering images using 12.8x fewer rays than NeRF approaches that render each pixel with a separate ray, allowing for important reductions in the use of memory and in computational complexity and enables the model to render large image patches at training time. We experiment with greater downsampling factors, but find that further increasing them causes 3D consistency artifacts.

In the presence of calibration and localization noise during training, we observe that NeRF models tend to generate blurry results which are particularly evident on dynamic objects where calibration and localization errors are compounded with errors in the estimation of the object pose. We ascribe this phenomenon to the use of reconstruction losses based on L2 distance which, in the presence of a color mismatch between the ground truth and the reconstructed pixel caused by input noise, favors the prediction of intermediate color values, generating blur. Using a feature renderer provides two advantages over the traditional approach. First, thanks to convolutional filters, the prediction for the feature associated to the current position can take into account the values of neighboring positions, enabling the model to produce a coherent output. Second, the possibility to render large patches makes it possible to adopt losses different from L2 distance, such as the perceptual loss of \emph{Johnson} \etal \cite{johnson2016perceptual} which penalizes more effectively implausible predictions such as the ones containing blur.

\begin{figure}
     \centering

     \includegraphics[width=1.0\linewidth]{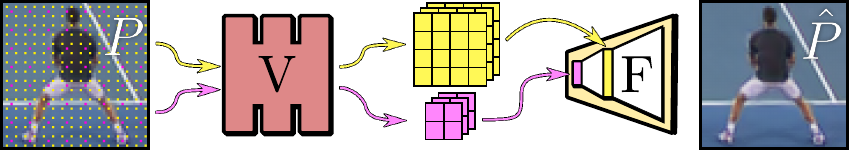}
     \caption{Representation of the feature rendering process. We sample points on rays arranged in a grid corresponding to feature map locations, then the sampled points are rendered into feature maps using our NeRF pipeline. The process is repeated to produce feature maps at different resolutions. The feature rendered $F$ uses the rendered feature maps to reconstruct the original image.}

    \label{fig:feature_renderer}
\end{figure}

\subsection{Object Configurations}
\label{sec:object_configurations}
On the \emph{Minecraft} dataset, we model the scene using four objects. The first object models the static scene elements close to the players, the second object models the distant objects and the other two objects model the players. For each ray, we sample 16 positions for the first model, 1 position for the second model and 32 positions for each of the players.

On the \emph{Tennis} dataset, we note that camera movement in the input dataset is mostly limited to camera rotations. Recovering depth information for the static objects is thus an ill-posed problem which requires prior knowledge. Note that this problem is not present for the players since their change of position with respect to the camera allows the learning of depth information. We thus adopt the following objects to model the environment: an object to model the tennis field which is bounded by a box $\beta$ that does not rise above ground level, an object to model the backplate of the tennis field, which is bounded by its box $\beta$ to be a planar surface, and two objects for the players. For each ray, we sample 4 positions for the objects modeling the static scene and 32 positions for each player.

\noindent\textbf{Minecraft Background Modeling}
The \emph{Minecraft} dataset features a challenging environment with distant visible objects. NeRF++ \cite{kaizhang2020nerfplusplus} employs an inverted sphere scene background representation for modeling distant objects. While effective, this parametrization requires a large number of samples to model distant objects, which increases memory consumption. To address this issue, we propose to model background objects using a spheric background representation which requires a single sample for each ray. In particular, we model the spheric background with as an MLP $f = V(d, o)$, receiving as input the direction $d$ and the origin $o$ of the ray, and returning as output the associated feature. We consider the opacity $\sigma$ of the associated feature to always be 1. The parametrization on the ray origin allows the model to simulate the effects of depth on the background objects without requiring multiple samples.

\subsection{Model Sharing}
\label{sec:model_sharing}
Instead of using a synthesis and an action module specific to each object, we note that objects corresponding to the same class can, in principle, be represented by the same model. In particular, in the \emph{Minecraft} dataset, the two players have completely symmetric characteristics, so we model both using a single shared model. While the same observation can be made for the case of the players in the \emph{Tennis} dataset, we found that the synthesis module fails if the same model is used for both players. We explain this behavior by observing that on the \emph{Tennis} dataset the player closest to the camera is always observed from the back, while the player further from the camera is always observed from the front. This asymmetry makes it harder for a model to learn a unified player representation, so we model the players with separate models.

\subsection{Masked Batch Normalization and Pooling}
\label{sec:masking}
In a video sequence, detection may fail in some frames. In the action module, the environment state corresponding to frames with missing detections and the successive ones are replaced with placeholder values. As discussed in Sec.~\ref{sec:action_training}, loss masking is used to prevent effects of placeholder values on training. Nevertheless, the presence of placeholder values may still alter the behavior of the action module by affecting the estimation of batch statistics in batch normalization layers and by affecting the behavior of operations such as global average pooling. To prevent potential undesired effects on training, in the action module we adopt masked versions of batch normalization and of pooling operations that operate by computing statistics only on non-placeholder values.
 
\section{Training details}
\label{sec:training}

In this section, we describe training details for the synthesis (see Sec.~\ref{sec:synthesis_training}) and the action modules (see Sec.~\ref{sec:action_training}).

\subsection{Synthesis module Training Details}
\label{sec:synthesis_training}
We optimize the synthesis module parameters using Adam \cite{kingma2014adam} as optimizer and learning rate $5e-4$. The model is trained for 300.000 iterations and the learning rate is exponentially decayed until $5e-5$ at the end of training. We employ a batch size of 8 video sequences, each with 3 or 4 frames for \emph{Minecraft} and \emph{Tennis} respectively. To better disentangle style from pose (see Sec.~3.3 on the main paper) we do not use consecutive frames for each sequence, but skip 4 and 100 frames between each selected frame respectively for \emph{Minecraft} and \emph{Tennis}.
 
In all the experiments, we consider input images of size 512x288 and we render patches of size 192x192 and 256x256 respectively for \emph{Minecraft} and \emph{Tennis} during training. To improve the quality of playable objects, we sample with increased frequency patches that contain the players.

The total loss is the weighted sum of the perceptual and L2 reconstruction losses in pixel space. We assign a weight of 1.0 to the L2 reconstruction loss and a weight of 0.1 to the perceptual loss term.

The synthesis module is trained on 4x Nvidia RTX 8000. We also train models on 1x Nvidia RTX 8000 on the \emph{Tennis} dataset using a reduced rendered patch size of 160x160 pixels with a small reduction in image quality.

\noindent\textbf{Feature Renderer Pretraining. } While it is possible to learn the feature renderer network $F$ from scratch, we find it beneficial to start training from pretrained weights since this guides the composable NeRF model towards learning features encodings whose mapping to the image space is already known. We obtain these weights with a pretraining process. We add a temporary encoder ConvNet to $F$ and train it as an autoencoder, using the same combination of perceptual and L2 losses used for training of the synthesis module. To avoid disruption of the learned features in the early stage of training of the synthesis module, we freeze $F$ during the first training iterations of the full model and unfreeze it once the composable NeRF model features become close to the ones the temporary ConvNet encoder would have produced.

\subsection{Action module Training Details}
\label{sec:action_training}
For the action module, we make use of Adam \cite{kingma2014adam} as optimizer with $\beta_1=0.5$ and $\beta_2=0.999$, and use a learning rate of $5e-4$. We train the model for 300.000 iterations with an exponentially decayed learning rate which reaches the value of $5e-5$ at the end of training. The action module and the discriminator are optimized in alternation. We regularize the discriminator training using spectral normalization \cite{miyato2018spectral}.

We note that at inference time our autoregressive dynamics network receives as input sequences of reconstructed environment states $\hat{s}_t$ rather than environment states $s_t$ produced by $E$ as happens during training. Following \cite{menapace2021pvg}, to avoid performance degradation at inference time due to this mismatch, we propose to train the action module using as input to the dynamics network encoded environment states for the first $t$ steps and reconstructed environment states for the following ones. In all the experiments we use 4 initial encoded environment states.

In addition, we employ a curriculum learning strategy where we linearly increase the length of the reconstructed sequences during training. In particular, at the beginning of training, sequences of 5 environment states are reconstructed, while at the end of the annealing period at step 25.000 the reconstructed sequence length is set to 9. We use a batch size of 64 sequences.

Following \cite{menapace2021pvg}, we set the number of actions $K$ to 7 for all the experiments.

We set $\lambda_\mathrm{rec}=1.0$, $\lambda_\mathrm{act}=0.15$, $\lambda_{\Delta}=0.1$ and $\lambda_{\mathrm{G}}=0.1$ in the computation of the total loss term.

The action module is trained on 1x Nvidia RTX 8000.

\noindent\textbf{Loss masking.}
During training of the action module, some frames may not contain a valid detection for each playable object. This may be due to the absence of the object in the frame or due to missed detections. We address this issue by computing the loss terms $\mathcal{L}_{\textrm{rec}}$, $\mathcal{L}_{\textrm{act}}$ and $\mathcal{L}_{\Delta}$ by taking into account only the prefix of the input sequence where the object has always been detected.

 %\willi{Describe ray patching for dynamic objects}
 %\willi{Experiments with rendering at increased resolution}
 %\willi{No hierarchical sampling for speed, describe nerf basics more in depth, eg approximation of the integral}
 %\willi{We rotate the bounding boxes to match the camera orientation}
