# Supplementary material for: Playable Environments: Video Manipulation in Space and Time
Source: arXiv:2203.01914 source file (2022-03-15)
Supplement: Supplementary file 5 [file supplementary_intro.tex]

In this Supplementary Material, we discuss additional implementation details (see Sec.~\ref{sec:implementation}), training details (see Sec.~\ref{sec:training}), provide details on the proposed datasets (see Sec.~\ref{sec:datasets}) and show additional experimental results (see Sec.~\ref{sec:experiments}). This Supplementary Material is complemented by a website (see \href{\webpage}{\webpagename}) showing additional video qualitative results such as sequences produced interactively by users, camera manipulation and style manipulation results. We also submit our code for review which will be made publicly available.
